# Supplementary material for: Update Rate, Accuracy, and Age of Information in a Wireless Sensor Network
Source: arXiv:2405.03798 source file (2024-05-06)
Supplement: Supplementary file 1 [file appendix.tex]

%\chapter{Evaluation of the Normalized Sum AoI (NSAoI)}
%In this Appendix, we first prove that the expression for $\mathbb E[L^2]$ in Eq.~\eqref{EL2} converges. Then we derive a lower bound on the NSAoI as given in Eq.~\eqref{NSAoI_EL} . %The lower bound can be made tighter by increasing the parameter $l_s$.

% \newpage
\section{Proof of convergence of $E[L^2]$}
% \texorpdfstring{$\mathbb E[L^2]$}{}}
\label{sec:a1}
In this Appendix, we prove that the expression for $\mathbb E[L^2]$ in Eq.~\eqref{EL2} converges. %and then we derive a upper bound on the absolute difference between the true value and the value if the upper limit of the sum is $l_s$.

Recall that
\begin{equation*}
    \mathbb E[L^2]=\sum_{l=1}^{\infty} P_{L}(l) \cdot l^2, \tag{\ref{EL2}}
\end{equation*}
where
\begin{small}
\begin{equation*}
    P_L(l)=\left[\left(\frac{q}{p}\right)^{\frac{T}{2}}+ \left(\frac{q}{p} \right)^{-\frac{T}{2}} \right] \frac{\sqrt{p q} }{T} \sum_{\nu=1}^{2T-1} \frac{(-1)^{\nu+1} \sin \left(\frac{\nu \pi}{2}\right) \sin \left(\frac{\nu \pi}{2T}\right)}{(s_{\nu})^{l-1}},\tag{\ref{pl}} 
\end{equation*}
\end{small}
and
\begin{equation*}
    s_{\nu}=\frac{1}{1-p-q+2 \sqrt{p q}\cos\left(\frac{\nu \pi}{2T}\right)},\quad \nu=1,2, \ldots, 2T-1. \tag{\ref{sv_T}} 
\end{equation*}
    
Substituting Eq.~\eqref{pl} into Eq.~\eqref{EL2}, we have
\begin{small}
\begin{align}
\mathbb E[L^2] =&\frac{\sqrt{p q} }{ T} \left(\left(\frac{q}{p}\right)^{\frac{T}{2}}+ \left(\frac{q}{p} \right)^{-\frac{T}{2}} \right) \sum_{l=1}^{\infty} \sum_{\nu=1}^{2 T-1} \frac{(-1)^{\nu+1} \sin \left(\frac{\nu \pi}{2}\right) \sin \left(\frac{\nu \pi}{2 T}\right)}{s_{\nu}^{l-1}} \cdot l^2 \notag \\
=&\frac{\sqrt{p q} }{ T}\left(\left(\frac{q}{p}\right)^{\frac{T}{2}}+ \left(\frac{q}{p} \right)^{-\frac{T}{2}} \right)  \sum_{\nu=1}^{2 T-1} \sum_{l=1}^{\infty} \frac{(-1)^{\nu+1} \sin \left(\frac{\nu \pi}{2}\right) \sin \left(\frac{\nu \pi}{2 T}\right)}{s_{\nu}^{l-1}} \cdot l^2 \notag \\
=& \frac{\sqrt{p q} }{T}\left(\left(\frac{q}{p}\right)^{\frac{T}{2}}+ \left(\frac{q}{p} \right)^{-\frac{T}{2}} \right)  \sum_{\nu=1}^{2 T-1} (-1)^{\nu+1} \sin \left(\frac{\nu \pi}{2}\right) \sin \left(\frac{\nu \pi}{2 T}\right)
\sum_{l=1}^{\infty} \frac{1}{s_{\nu}^{l-1}} \cdot l^2 \label{EL-sum}
%=&\frac{\sqrt{p q} }{ T}\left(\left(\frac{q}{p}\right)^{\frac{T}{2}}+ \left(\frac{q}{p} \right)^{-\frac{T}{2}} \right) \left( \sum_{l=1}^{\infty} \frac{(-1)^{2} \sin \left(\frac{ \pi}{2}\right) \sin \left(\frac{\pi}{2 T}\right)}{s_{1}^{l-1}} \cdot l^2 \right. \notag \\
%& \left. + \sum_{l=1}^{\infty} \frac{(-1)^{3} \sin \left(\frac{2 \pi}{2}\right) \sin \left(\frac{2 \pi}{2 T}\right)}{s_{2}^{l-1}} \cdot l^2 \right. \left. + \cdots + \sum_{l=1}^{\infty} \frac{(-1)^{2 T} \sin \left(\frac{(2T-1) \pi}{2}\right) \sin \left(\frac{(2T-1) \pi}{2 T}\right)}{s_{2T-1}^{l-1}} \cdot l^2 \right) \notag \\
%=& \frac{\sqrt{p q} }{T}\left(\left(\frac{q}{p}\right)^{\frac{T}{2}}+ \left(\frac{q}{p} \right)^{-\frac{T}{2}} \right) \left[ (-1)^{2} \sin \left(\frac{ \pi}{2}\right) \sin \left(\frac{\pi}{2 T}\right) \sum_{l=1}^{\infty} \frac{l^2}{s_{1}^{l-1}} \right. \notag \\
%& \left. +(-1)^{3} \sin \left( \pi \right) \sin \left(\frac{\pi}{T}\right) \sum_{l=1}^{\infty} \frac{l^2}{s_{2}^{l-1}} + \cdots  \right. \notag \\
%&\left. +(-1)^{2 T} \sin \left(\frac{(2T-1) \pi}{2}\right) \sin \left(\frac{(2T-1) \pi}{2 T}\right) \sum_{l=1}^{\infty} \frac{l^2 }{s_{2T-1}^{l-1}} \right] \label{EL2_1}
\end{align}
\end{small}
From Eq.~\eqref{EL-sum}, we can see that $\mathbb E[L^2]$ is expressed as the sum of $2T-1$ infinite sums. 

We now prove that each infinite sum in Eq.~\eqref{EL2} converges. %, and we derive a lower bound for each infinite series.
For notation simplicity, let 
\begin{equation}
    \alpha_{\nu} = \frac{1}{s_{\nu}}= 1-p-q+2 \sqrt{p q}\cos\left(\frac{\nu \pi}{2T}\right), \quad \nu=1,2, \cdots, 2T-1.
\end{equation}
Then 
\begin{equation}
    \mathbb E[L^2] =\frac{\sqrt{p q} }{T}\left(\left(\frac{q}{p}\right)^{\frac{T}{2}}+ \left(\frac{q}{p} \right)^{-\frac{T}{2}} \right) \sum_{\nu=1}^{2T-1} C_{\nu} \sum_{l=1}^{\infty} l^2 \alpha_{\nu}^{l-1},\label{EL2_2}
\end{equation}
where 
\begin{equation}
    C_{\nu} = (-1)^{\nu+1} \sin \left(\frac{\nu \pi}{2}\right) \sin \left(\frac{\nu \pi}{2 T}\right).
    \label{Cv}
\end{equation}
As $\mathbb E[L^2]$ is the sum of $\sum_{l=1}^{\infty} \alpha_{\nu}^{l-1} l^2$ with different coefficients, we want to prove $\sum_{l=1}^{\infty} \alpha_{\nu}^{l-1} l^2$ converges for any value of $\nu \in \{1,2,\cdots,2T-1\}$.

\newenvironment{claim}[1]{\par\noindent\textbf{Claim 1.}\space#1}{}
\begin{claim}
    $-1<\alpha_{\nu}<1$, where $\nu=1,2, \cdots, 2T-1$. $T$ is a given positive integer.
\end{claim}
\begin{proof}
Given \(0 \leq p \leq 1, 0 \leq q \leq 1 \text{, and } 0 \leq p+q \leq 1\), we have
\begin{align*}
1-\alpha_{\nu}&=p+q-2 \sqrt{p q}\cos\left(\frac{\nu \pi}{2T}\right)\\
&=(\sqrt{p}-\sqrt{q})^2+2\sqrt{p q} \left( 1- \cos \left(\frac{\nu \pi}{2T}\right) \right).
\end{align*}
Since $0<\frac{\nu \pi}{2T}<\pi$, 
$1-\cos\left(\frac{\nu \pi}{2T}\right)>0$. Thus, $1-\alpha_{\nu}>0, \alpha_{\nu}<1.$
Similarly,
\begin{align*}
1+\alpha_{\nu}&=2-p-q+2\sqrt{p q}\cos \left(\frac{\nu \pi}{2T}\right) \\
&> 2-p-q-2\sqrt{p q} \\
&= 2-(\sqrt{p}+\sqrt{q})^2.
\end{align*}
Since $(\sqrt{p}+\sqrt{q})^2$ reaches its maximum value of 2 when $p=q=0.5$, $2-(\sqrt{p}+\sqrt{q})^2 \geq 0$. Thus, $1+\alpha_{\nu}>0$, $\alpha_{\nu}>-1$.
\end{proof}

\newenvironment{claim2}[1]{\par\noindent\textbf{Claim 2.}\space#1}{}
\begin{claim2}
    The infinite sum $\sum_{l=1}^{\infty} \alpha_{\nu}^{l-1}\cdot l^2$ converges for any $\nu \in \{1,2, \cdots, 2T-1\}$.
\end{claim2}
\begin{proof}
%Let $a_l=\alpha_{\nu}^{l-1}\cdot l^2$. 
For any $\nu \in \{1,2, \cdots, 2T-1\}$, $-1<\alpha_{\nu}<1$.\\
%If $\alpha_{\nu} = 0$, $\sum_{l=1}^{\infty} \alpha_{\nu}^{l-1}\cdot l^2$ converges to 0.\\
%If $\alpha_{\nu} \in (-1,0) \cup (0,1)$, 
%For any $\nu$, $\alpha_{\nu}$ is fixed and known.
%We prove $\sum_{l=1}^{\infty} a_L$ converges, i.e., $\lim_{L \to \infty} a_L =0$.
We perform a ratio test \cite{infinite} to examine the convergence:
\begin{align}
%\lim_{l\to\infty} \left| \frac{a_{l+1}}{a_{l}} \right|
\lim_{l\to\infty} \left| \frac{\alpha_{\nu}^l \cdot (l+1)^2}{\alpha_{\nu}^{l-1} \cdot l^2} \right| \notag 
&= \lim_{l\to\infty} \left| \alpha_{\nu}\cdot \left( 1+\frac{2}{l}+\frac{1}{l^2} \right) \right| \notag \\
&= \left| \alpha_{\nu} \right|.
\end{align}
If this limit is smaller than 1, the sum converges absolutely \cite{infinite}. Since $\left| \alpha_{\nu} \right|<1$, $\sum_{l=1}^{\infty} \alpha_{\nu}^{l-1}\cdot l^2$ converges.
%which tells us that $\sum_{l=1}^{\infty} \alpha_{\nu}^{l-1}\cdot l^2$ is absolutely convergent \cite{infinite}.\\

Thus $\sum_{l=1}^{\infty} \alpha_{\nu}^{l-1}\cdot l^2$ converges for any $\nu \in \{1,2, \cdots, 2T-1\}$. 
%!!The closer $\alpha_{\nu}$ to 1 is, the more slowly this sum converges.
\end{proof}
From Eq.~\eqref{Cv}, we note that $C_{\nu}$ is a finite real number. Then $ C_{\nu} \sum_{l=1}^{\infty} \alpha_{\nu}^{l-1}\cdot l^2$ converges and so does $\mathbb E[L^2]$.
%, and thus the finite sum of $\sum_{l=1}^{\infty} \alpha_{\nu}^{l-1}\cdot l^2$ multiplied by a constant factor is still convergent \cite{infinite}, i.e., $\mathbb E[L^2]$ is convergent.

\section{Evaluation of NSAoI}
\label{sec:a2}
In this Appendix, we derive a lower bound on the NSAoI. The lower bound can be made tighter by increasing the upper limit $l_s$ of the sum in Eq.~\eqref{EL2}.

Recall that
\begin{equation*}
    \text{NSAoI}=\frac{1}{2} \left(1+\frac{\mathbb E[L^2]}{\mathbb E[L]} \right),  \tag{\ref{NSAoI_EL}} 
\end{equation*}
where $\mathbb E[L]$ is given in Eq.~\eqref{EL}, and is a constant for given values of $T,p,q$.
%Since $\mathbb E[L^2]$ is proved to be convergent, NSAoI converges to a real number. We can obtain NSAoI by estimating $\mathbb E[L^2]$.

From Eq.~\eqref{EL2_2}, we need to evaluate each infinite sum $\sum_{l=1}^{\infty} l^2 \alpha_{\nu}^{l-1}$, for $\nu \in \{1,2, \cdots, 2T-1\}$.
%Suppose the series converges to $\Sigma_{\nu}$, i.e.,
Let
\begin{equation}
    \Sigma=\sum_{l=1}^{\infty}\alpha_{\nu}^{l-1} \cdot l^2.
\end{equation}
Let the partial sum be
\begin{equation}
    \Sigma_{l_s}=\sum_{l=1}^{l_s}\alpha_{\nu}^{l-1} \cdot l^2
\end{equation}
%Then the limit of the partial sum is $\Sigma_{\nu}$. In other words,
so that
\begin{equation}
    \lim_{l_s \to \infty} \Sigma_{l_s} = \Sigma.
\end{equation}
Since $\Sigma_{l_s}$ converges, the partial sum, $\Sigma_{l_s}$ can be made arbitrarily close to $\Sigma$ by taking a sufficient large $l_s$. %Therefore, we take a partial sum and use that as an estimation of the value of the series and discuss how good the estimation is.

Let %the remainder denoted by $R_{\nu,n}$.
\begin{equation}
    R_{l_s} \triangleq \Sigma-\Sigma_{l_s}=\sum_{l=l_s+1}^{\infty}\alpha_{\nu}^{l-1} \cdot l^2
\end{equation}
denote the error between the exact value of the series and the partial sum with $l_s$ terms. We next derive a bound on $R_{l_s}$. %to assess how good the estimation is.

If $0 \leq \alpha_{\nu} <1$, $\alpha_{\nu}^{l-1}\cdot l^2$, $l=1,2,\cdots$, is non-negative. However, if $-1 < \alpha_{\nu}<0$, $\alpha_{\nu}^{l-1}\cdot l^2$, $l=1,2,\cdots$, is a series with alternating positive and negative values.
Therefore, we consider the two cases separately.
\begin{itemize}
    \item Case 1. $0 \leq \alpha_{\nu} <1$:\\
    Let %$f_{}(x)$, where
    \begin{equation}
        f_{}(x)=\alpha_{\nu}^{x-1}\cdot x^2.
    \end{equation} 
    The integral of $f_{}(x)$ is calculated by using ``int" command in Maple software as
    \begin{equation}
        \int f_{}(x)\,d x
        = \frac{\alpha_{\nu}^{x-1} \left( x^2 \ln^2{\alpha_{\nu}}-2x \ln{\alpha_{\nu}}+2 \right)}{\ln^3{\alpha_{\nu}}}. \label{int-f}
    \end{equation}

\begin{figure}[h]
\centering
\includegraphics[scale=0.5]{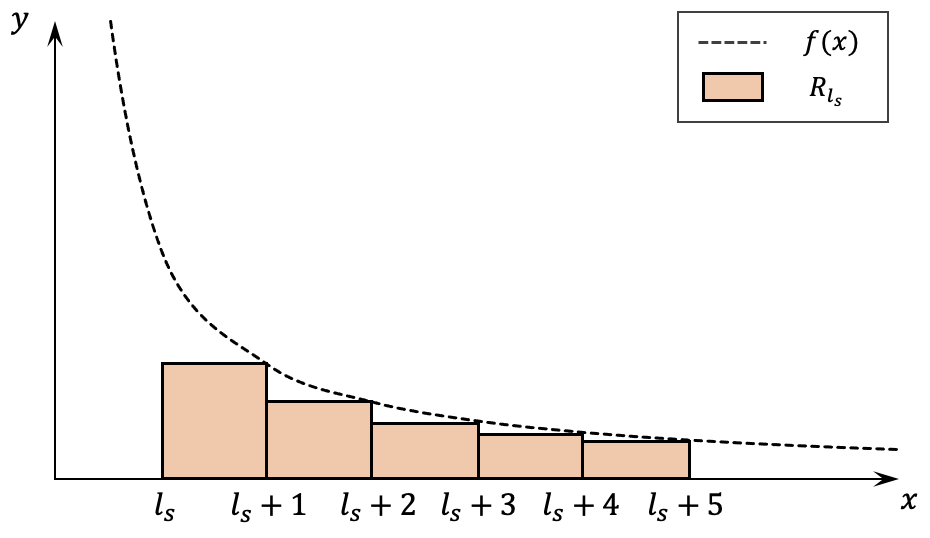}
\caption{An illustration of the curve $f_{}(x)$ on $[l_s,\infty)$ and the remainder $R_{l_s}$.}
\label{fig:under}
\end{figure}

As shown in Figure~\ref{fig:under}, if we take rectangles of width 1 and use the right endpoint as the height of the rectangle starting from $x=l_s$, we can write %the area under $f_{}(x)$ on $[n,\infty)$. This estimation is the remainder $R_{\nu,n}$, and it underestimate the area under the curve of $f_{}(x)$ on the interval $[n,\infty]$.
%And $R_{\nu,n}$ could also be viewed as an overestimation of $f_{}(x)$ on interval $[n+1,\infty]$.
%That is,
    \begin{equation}
    \begin{aligned}
        R_{l_s} \leq \int_{l_s}^{\infty}f_{}(x)\,d x.
    %\int_{n+1}^{\infty}f_{}(x)\,d x \leq R_{\nu,n} \leq \int_n^{\infty}f_{}(x)\,d x
    \end{aligned}
    \end{equation}
From Eq.~\eqref{int-f}, we have
\begin{small}
\begin{align}
\int_{l_s}^{\infty}f_{}(x)\,d x &= \frac{\displaystyle \lim_{x\to\infty} \alpha_{\nu}^{x-1} \left( x^2 \ln^2{\alpha_{\nu}}-2x \ln{\alpha_{\nu}}+2 \right) - 
    \alpha_{\nu}^{l_s-1} \left( {l_s}^2 \ln^2{\alpha_{\nu}}-2l_s \ln{\alpha_{\nu}}+2 \right)}
    {\ln^3{\alpha_{\nu}}}\notag \\
    &=-\frac{\alpha_{\nu}^{l_s-1} \left( {l_s}^2 \ln^2{\alpha_{\nu}}-2l_s \ln{\alpha_{\nu}}+2 \right)}{\ln^3{\alpha_{\nu}}}, \label{fn}
\end{align}
\end{small}

where $\lim_{x\to \infty} \alpha_{\nu}^x x^2$ $=\lim_{x\to \infty} \alpha_{\nu}^x x$ $=\lim_{x \to \infty} \alpha_{\nu}^x=0$ as $\alpha_{\nu}<1$.

Similarly, if we take rectangles of width 1 and use the left endpoint as the height of the rectangle starting from $x=l_s+1$, %which gives an estimation of the area under $f_{}(x)$ on the interval $[n+1,\infty)$. This 
as shown in Figure~\ref{fig:over}, we can write
%see that $R_{\nu,n}$ is this estimation and can be viewed as an overestimation of the area under the curve of $f_{}(x)$ on the interval $[n+1,\infty]$, i.e.,
\begin{equation}
    R_{l_s} \geq \int_{l_s+1}^{\infty}f_{}(x)\,d x.
\end{equation}
From Eq.~\eqref{int-f}, we have
\begin{small}
\begin{align}
\int_{l_s+1}^{\infty}f_{}(x)\,d x &= \frac{\displaystyle \lim_{x\to\infty} \alpha_{\nu}^{x-1} \left( x^2 \ln^2{\alpha_{\nu}}-2x \ln{\alpha_{\nu}}+2 \right) - 
\alpha_{\nu}^{l_s} \left[(l_s+1)^2 \ln^2{\alpha_{\nu}}-2(l_s+1) \ln{\alpha_{\nu}}+2 \right]}
{\ln^3{\alpha_{\nu}}}\notag \\
&=-\frac{\alpha_{\nu}^{l_s} \left[ (l_s+1)^2 \ln^2{\alpha_{\nu}}-2(l_s+1) \ln{\alpha_{\nu}}+2 \right]}{\ln^3{\alpha_{\nu}}}. \label{fn+1}
\end{align}
\end{small}
\begin{figure}[!t]
\centering
\includegraphics[scale=0.5]{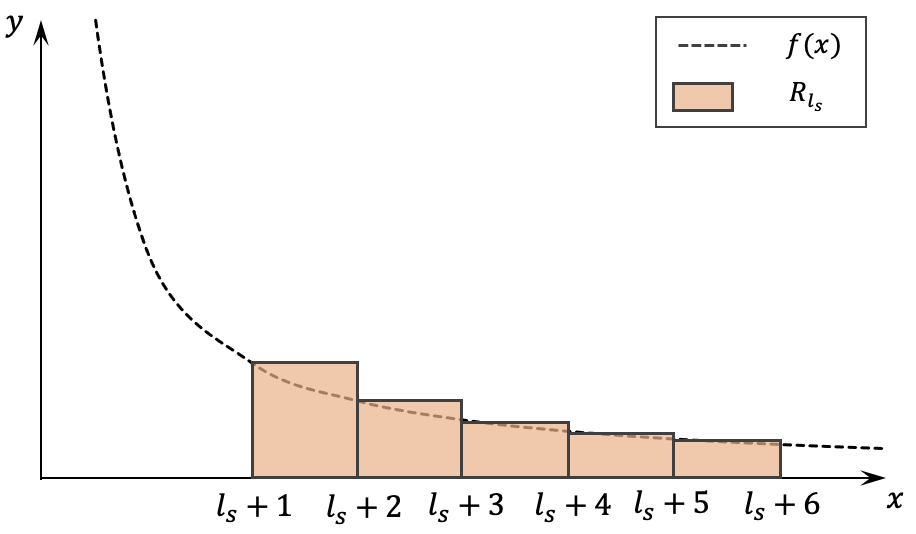}
\caption{An illustration of the curve $f_{}(x)$ on $[l_s+1,\infty)$ and the remainder $R_{l_s}$.}
\label{fig:over}
\end{figure}

Therefore,
\begin{equation}
    \int_{l_s+1}^{\infty}f_{}(x)\,d x \leq R_{l_s} \leq \int_{l_s}^{\infty}f_{}(x)\,d x, \label{Rvn}
\end{equation}
where $\int_{l_s+1}^{\infty}f_{}(x)\,d x$ is given in Eq.~\eqref{fn+1} and $\int_{l_s}^{\infty}f_{}(x)\,d x$ is given in Eq.~\eqref{fn}.

\item Case 2. $-1 < \alpha_{\nu}<0$:\\
%Let $b_{l}= \left( -\alpha_{\nu} \right)^{l-1}  \cdot l^2$. 
%Then 
%\begin{equation}\sum_{l=1}^{\infty}\alpha_{\nu}^{l-1} \cdot l^2 = \sum_{l=1}^{\infty} (-1)^{l-1} b_l.
%\end{equation}
%Then $b_{l}$ has the same numerical values as $\alpha_{\nu}^{l-1} \cdot l^2$, but they are all positive.
%Perform a ratio test on $b_{l}$:
%\begin{align}
    %\lim_{l\to\infty} \left| \frac{b_{l+1}}{b_{l}} \right| \notag 
%&= \lim_{l\to\infty} \left| \frac{(-\alpha_{\nu})^l \cdot (l+1)^2}{(-\alpha_{\nu})^{l-1} \cdot l^2} \right| \notag \\
%&=\lim_{l\to\infty} \left| (-\alpha_{\nu})\cdot \left( 1+\frac{2}{l}+\frac{1}{l^2} \right) \right| \notag \\
%&= \left| -\alpha_{\nu} \right|<1.
%\end{align}
According to the ratio test, $\sum_{l=1}^{\infty}\alpha_{\nu}^{l-1} \cdot l^2$ converges eventually, i.e., $\alpha_{\nu}^{l-1} \cdot l^2$ decreases in numerical value for a large $l$, but may increase in numerical value when $l$ is small. Assume that for $l < l_d$, $l_d \in \{1,2,\cdots\}$, $\alpha_{\nu}^{l-1} \cdot l^2$ increases in numerical value, and for $l \geq l_d$, $\alpha_{\nu}^{l-1} \cdot l^2$ decreases in numerical value. Then we have
\begin{equation}
    \Sigma= \sum_{l=1}^{\infty}\alpha_{\nu}^{l-1} \cdot l^2 = \sum_{l=1}^{l_d}\alpha_{\nu}^{l-1} \cdot l^2 + \sum_{l_d}^{\infty}\alpha_{\nu}^{l-1} \cdot l^2.
\end{equation}

%Since $-1 < \alpha_{\nu}<0$, $b_{l}>0$. 
Since $\sum_{l_d}^{\infty}\alpha_{\nu}^{l-1} \cdot l^2$ converges and its terms in never increase in numerical value, the exact value of the sum $\Sigma$ lies between $\Sigma_{l_s}$ and $\Sigma_{l_s+1}$ for any $l_s \geq l_d$ \cite{infinite}, i.e.,
% \begin{small}
\begin{align}
    \left|R_{l_s}\right| &= \left|\Sigma-\Sigma_{l_s}\right| \leq\left|\Sigma_{l_s+1}-\Sigma_{l_s}\right|
    =|\alpha_{\nu}^{l_s}\cdot (l_s+1)^2|\notag \\
    &=(-\alpha_{\nu})^{l_s}\cdot (l_s+1)^2,  l_s \geq l_d. \label{Rvn2}
\end{align}
% \end{small}
%$\sum_{l=1}^{\infty} a_L$ becomes an alternative series, and its convergent series is $\sum_{l=1}^{\infty} (-1)^{L} b_{L}$, where $b_{L}= \left( -\alpha_{\nu} \right)^{l-1}  \cdot l^2$. It is obvious that $b_L>0$, and is decreasing. $\Sigma$ lies between $\Sigma_n$ and $\Sigma_{n+1}$ for any $n$. 
% Why s lies between s_n and s_{n+1}? Or find some reference. solved
\end{itemize}
Therefore, we obtain a lower bound and an upper bound for $R_{l_s}$ when $0 \leq \alpha_{\nu} <1$, and we obtain an upper bound on $R_{l_s}$ when $-1 < \alpha_{\nu}<0$. These bounds are used to derive an upper bound on $R_{L^2}$, which denotes the error on estimating $\mathbb E[L^2]$ using $\sum_{l=1}^{l_s} P_{L}(l) \cdot l^2$. That is
%$R_\text{NSAoI}$, which denotes the error between the exact value of the NSAoI and the NSAoI calculated using partial sum $\sum_{l=1}^{n} P_{L}(l) \cdot l^2$ for $\mathbb E[L^2]$ in Eq.~\eqref{NSAoI_EL}.

%Since $\nu \in [1,2T-1]$, $\frac{\nu \pi}{2 T} \in \left[\frac{\pi}{2T},\frac{(2T-1)\pi}{2T}\right] \in [0,\pi]$. Since $f=\cos(x)$ is a decreasing function of $x$ on $[0,\pi]$, $\alpha_{\nu}$ is a decreasing function of $\nu$. %Then there exist an integer $v \in [1,2T-1]$   that makes $\alpha_{\nu} \geq 0$ when $\nu \leq v$ and $\alpha_{\nu} < 0$ when $\nu > v$
\begin{equation}
    R_{L^2} = \sum_{l=1}^{\infty} P_{L}(l) \cdot l^2 - \sum_{l=1}^{l_s} P_{L}(l) \cdot l^2 \geq 0. \label{Rn}
\end{equation}
From Eqs.~\eqref{EL2_2},~\eqref{Rvn},~\eqref{Rvn2},~\eqref{Rn}, we have
\begin{small}
\begin{align}
    R_{L^2} &= \frac{\sqrt{p q} }{T}\left(\left(\frac{q}{p}\right)^{\frac{T}{2}}+ \left(\frac{q}{p} \right)^{-\frac{T}{2}} \right) \left( \sum_{\nu=1}^{2T-1} C_{\nu} \sum_{l=1}^{\infty} l^2 \alpha_{\nu}^{l-1} - \sum_{\nu=1}^{2T-1} C_{\nu} \sum_{l=1}^{l_s} l^2 \alpha_{\nu}^{l-1} \right) \notag \\
    &=\frac{\sqrt{p q} }{T}\left(\left(\frac{q}{p}\right)^{\frac{T}{2}}+ \left(\frac{q}{p} \right)^{-\frac{T}{2}} \right) \sum_{\nu=1}^{2T-1} C_{\nu} \left(\sum_{l=1}^{\infty} l^2 \alpha_{\nu}^{l-1} - \sum_{l=1}^{l_s} l^2 \alpha_{\nu}^{l-1} \right) \notag \\
    &\leq \frac{\sqrt{p q} }{T}\left(\left(\frac{q}{p}\right)^{\frac{T}{2}}+ \left(\frac{q}{p} \right)^{-\frac{T}{2}} \right) \left( \sum_{\substack{\nu=1,2,...,2T-1,\\ \alpha_{\nu} \geq 0}} C_{\nu} B_{\nu} + \sum_{\substack{\nu=1,2,...,2T-1,\\ \alpha_{\nu}< 0}} | C_{\nu} (-\alpha_{\nu})^{l_s}\cdot (l_s+1)^2 | \right), \label{Rn_bound} %\left(\sum_{l=1}^{\infty} l^2 \alpha_{\nu}^{l-1} - \sum_{l=1}^{n} l^2 \alpha_{\nu}^{l-1} \right),
\end{align}
\end{small}
where $C_{\nu}$ is given in Eq.~\eqref{Cv}, and
\begin{equation}
    B_{\nu} = \left\{\begin{array}{ll}
\displaystyle -\frac{\alpha_{\nu}^{l_s-1} \left( l_s^2 \ln^2{\alpha_{\nu}}-2l_s \ln{\alpha_{\nu}}+2 \right)}{\ln^3{\alpha_{\nu}}}, %\int_n^{\infty}f_{}(x)\,d x, 
& \text {when } C_{\nu} \geq 0  \vspace{1ex} \\
\displaystyle -\frac{\alpha_{\nu}^{l_s} \left[ (l_s+1)^2 \ln^2{\alpha_{\nu}}-2(l_s+1) \ln{\alpha_{\nu}}+2 \right]}{\ln^3{\alpha_{\nu}}}, %\int_{n+1}^{\infty}f_{}(x)\,d x, 
& \text{when } C_{\nu}< 0
\end{array}\right.\label{Bv}
\end{equation}
A tighter upper bound on $R_{l_s}$ is obtained as $l_s$ is increased. From Eq.~\eqref{NSAoI_EL}, the error between the exact NSAoI and the estimated NSAoI calculated using estimated $\mathbb E[L^2]$ is given by
%, which tells us the difference between $\mathbb E[L^2]=\sum_{l=1}^{\infty} P_{L}(l) \cdot l^2$ and the estimation $\sum_{l=1}^{n} P_{L}(l) \cdot l^2$. By using this estimation in Eq.~\eqref{NSAoI}, we have the error between the exact NSAoI and the estimated NSAoI:
\begin{equation}
    R_{\text{NSAoI}} = \frac{1}{2} \cdot \frac{R_{L^2}}{\mathbb E [L]}.
    \label{R_NSAoI}
\end{equation}
From Eqs.~\eqref{Rn_bound},~\eqref{R_NSAoI}, $R_{\text{NSAoI}}$ can be upper bounded by $U_{\text{NSAoI}}$, i.e.,
\begin{align}
\begin{split}
    R_{\text{NSAoI}} \leq U_{\text{NSAoI}} = \frac{1}{2} +\frac{1}{2 \mathbb E [L]} \cdot \frac{\sqrt{p q} }{T}\left(\left(\frac{q}{p}\right)^{\frac{T}{2}}+ \left(\frac{q}{p} \right)^{-\frac{T}{2}} \right) \left( \sum_{\substack{\nu=1,2,...,2T-1,\\ \alpha_{\nu} \geq 0}} C_{\nu} B_{\nu} \right. \\
     \left.+ \sum_{\substack{\nu=1,2,...,2T-1,\\ \alpha_{\nu}< 0}} | C_{\nu} (-\alpha_{\nu})^{l_s}\cdot (l_s+1)^2 | \right) .
     \label{U_NSAoI}
\end{split}
\end{align}

For a desired maximum error $\epsilon$, i.e., $R_{\text{NSAoI}}<\epsilon$, we can calculate the smallest required value of $l_s$ using Eq.~\eqref{U_NSAoI}. 

By upper bounding $R_{\text{NSAoI}}$, we obtain a lower bound on the NSAoI, i.e.,
\begin{equation}
    \text{NSAoI}_{l_s} (T) = \frac{1}{2} \left(1+\frac{\sum_{l=1}^{l_s} P_{L}(l) \cdot l^2}{\mathbb E[L]} \right).
    \tag{\ref{NSAoI_ls}}
\end{equation}
The lower bound can be tightened by increasing the value of $l_s$.

%Assume it is required that the error between the exact NSAoI and the estimated NSAoI should be less than $e$. Then we can calculate the minimum upper limit $l_s=\min\{n \mid n \in Z_+ \text{, } U_n<e\}$ to ensure the accuracy.

\endinput

Recall that
\begin{equation*}
    \text{NSAoI}=\frac{1}{2} \left(1+\frac{\sum_{l=1}^{\infty} P_{L}(l) \cdot l^2}{\mathbb E[L]} \right),
    \tag{\ref{ENSAoI}}
\end{equation*}
where $P_{L}(l)$ is given in Eq.~\eqref{pk}.
Since $\mathbb E[L^2]=\sum_{l=1}^{\infty} P_{L}(l) \cdot l^2$. Then $\text{NSAoI}=\frac{1}{2} \left(1+\frac{\mathbb E[L^2]}{\mathbb E[L]} \right)$, where $\mathbb E[L]$ is given in Eq.~\eqref{EL}. Then we evaluate $\mathbb E[L^2]$.

Substituting $\alpha_{\nu}$, we have
\begin{equation}
\begin{aligned}
\mathbb E[L^2] &= \frac{\sqrt{p q} }{T}\left(\left(\frac{q}{p}\right)^{\frac{T}{2}}+ \left(\frac{q}{p} \right)^{-\frac{T}{2}} \right) \left[ \sin \left(\frac{ \pi}{2}\right) \sin \left(\frac{\pi}{2 T}\right) \sum_{l=1}^{\infty} l^2\alpha_{1}^{l-1}  - \sin \left( \pi \right) \sin \left(\frac{\pi}{T}\right) \sum_{l=1}^{\infty} l^2 \alpha_{2}^{l-1} \right. \\& \left. + \cdots + \sin \left(\frac{(2T-1) \pi}{2}\right) \sin \left(\frac{(2T-1) \pi}{2 T}\right) \sum_{l=1}^{\infty} l^2 \alpha_{2T-1}^{l-1} \right]
\label{N}
\end{aligned}
\end{equation}

\begin{equation}
\begin{aligned}
N_n &= \frac{\sqrt{p q} }{T}\left(\left(\frac{q}{p}\right)^{\frac{T}{2}}+ \left(\frac{q}{p} \right)^{-\frac{T}{2}} \right) \left[ \sin \left(\frac{ \pi}{2}\right) \sin \left(\frac{\pi}{2 T}\right) \sum_{l=1}^{n} l^2\alpha_{1}^{l-1}  - \sin \left( \pi \right) \sin \left(\frac{\pi}{T}\right) \sum_{l=1}^{n} l^2 \alpha_{2}^{l-1} \right. \\& \left. + \cdots + \sin \left(\frac{(2T-1) \pi}{2}\right) \sin \left(\frac{(2T-1) \pi}{2 T}\right) \sum_{l=1}^{n} l^2 \alpha_{2T-1}^{l-1} \right].
\end{aligned}
\end{equation}

Then \[\text{ENSAoI}_n=\frac{1}{2} \left(1+\frac{N_n}{\mathbb E[L]} \right),\]
\[\mid \text{ENSAoI}-\text{ENSAoI}_n \mid=\frac{| N-N_n|}{2 \mathbb E [L]}.
\]
%Since for two arbitrary real numbers $a,b$, $\mid a+b \mid <= |a| +| b|$.
For a fixed $n$, the absolute value, $|N-N_n|$ can be upper bounded by summing the upper bound of the absolute value of the remainder $R_{\nu,n}$ with positive coefficients for each term.
